# Supplementary material for: Chest ImaGenome Dataset for Clinical Reasoning
Source: arXiv:2108.00316 source file (2021-07-31)
Supplement: Supplementary file 1 [file supplementary_B.tex]

% useful but need more time to clean

\textbf{Vision Driving Chest ImaGenome Dataset's Construction}: In the Chest ImaGenome dataset, the goal for analyzing the CXR reports with NLP is to extract radiology knowledge in the form of an anatomically centered graph. To summarize, the aim of our dataset creation strategy is several fold, which is driven by the following clinical and technical rationale:

% Technically, why did we pick anatomies as objects in the scene graph
1. We wanted to propose a potentially scalable automatic approach (i.e. not restricted to CXR) in generating Visual-Genome-like datasets in the medical domain, where manual annotations are often prohibitively resource intensive and often can only be reserved for creating smaller gold standard datasets. By centering the object detection at the anatomic level, we could structure radiology reports to derive attribute(s) associated with different anatomies, and separately harness mature imaging atlas segmentation models for different modalities to detect these anatomical location(s) on the corresponding images. This approach has been previous shown to be successful in creating a locally labeled dataset for one attribute (lung opacity) in CXRs \cite{}, with which an object detection network using RetinaNet was trained that reached a similar performance level as networks trained on manually annotated datasets \cite{}. In this paper, we not only extend the work to more anatomical locations and CXR attributes, we also formally represented the annotations as a knowledge graph, which requires implementation of additional logic for consistency checking. Furthermore, all nodes in the CXR scene graphs have been linked to an external recognized medical ontology, the Unified Medical Language System (UMLS) \cite{}, to support downstream semantic and ontological reasoning tasks.

% We describe our dataset as 'scene-graph-like' because only the anatomical concept nodes in the graphs are true 'objects' that have corresponding bounding box coordinates on the image in the Visual Genome's sense. All abnormal findings and devices in CXR reports are expressed as attribute nodes related to the object nodes in our scene graphs. 
% The approach is limited by the extent of the NLP and the bbox extraction pipeline, both of which can be technically improved upon given the resource

% Why connecting information along anatomical lines makes sense clinically
2. Across multiple medical sub-specialties, with the appropriate ontology, descriptions of a patient's symptoms, diseases, treatments and even laboratory tests can be normalized to some medical attribute related to specific anatomies as measured at different time points. Structuring imaging attributes at anatomical levels would allow integration of pixel level information with the rest of the patient electronic record and with external medical ontologies (e.g. the UMLS \cite{}) in a way that could connect information across time and medical specialty domains. With CXR being a less specific screening type exam, connecting localized attributes (e.g. a right upper lung mass, a lower lobe consolidation, etc) with other sources of information about the attribute from another clinical modality if available (e.g. the pathology biopsy report for the lung mass, the patient's respiratory rate from vital sign records, etc) would greatly enrich what we know and can infer with the CXR images. Furthermore, many clinical exams, including CXRs, are repeated ordered to follow disease progression in response to different management pathways. These clinically relevant disease progression changes are examined and observed at the anatomical level. Therefore, in our dataset, these changes (improved, worsened, and no change) are represented as comparison relations between anatomical locations with respect to the describe CXR attribute(s).

% Our dataset's implication/advantages for fusion modeling
3. Clinicians often integrate clinical features along anatomical lines for various complex reasoning processes, including making differential diagnoses, making decisions about treatments, or giving disease progression prognosis. For example, in the CXR context, a visual observation of new or worsened pulmonary edema (in the lungs) and enlarged cardiac silhouette (heart) patterns on the image, in combination with e.g. symptoms of shortness of breath and physical exam findings of swelling in the legs, will likely lead a clinician to prescribe drugs for improving the functions of the anatomies causing these symptoms and ordering tests to track the progression of various anatomical functions (e.g. creatinine for kidneys, echocardiogram to measure the heart's ejection fraction, etc). In comparison, current multi-modal models in the medical domain typically blindly fuse features from different clinical modalities (data sources) without any intelligence added from domain specific knowledge. Since deep learning models are known to predict using spurious correlations between input features, the lack of clinical intelligence in fusion model development is a serious cause for concern. Therefore, the graph dataset we constructed is anatomy centered to provide plausible biological connections that could be suitable for supporting downstream multi-modal modeling purposes.

% Why our dataset is suitable for further creation of VQA like dataset for CXRs and why these VQA interactive models might be useful clinically
4. Lastly, we set out to create a graph dataset where the nodes and relations in the report-derived knowledge graphs actually constitute logically true or probable medical statements. This opens up the possibility of (semi-)automatically deriving simple clinical questions (because one would ideally want to check a subset for clinical relevance) from existing answers in the report knowledge graphs. A clinical application relevant Visual Question and Answer dataset would open up the possibility for training an interactive CXR interpretation system. Now, why would such a system be clinically useful? 
% need some help here Kashyap
In the non-medical domain, works in the visual question answering and natural language inference literature have seen applications in XYZ...  
% key advantages? is the VQA modeling framework more suited to assess how muc the model learn/rely on language priors and how much on the actual imaging findings?
In the clinical domain, consultations between clinicians who specialize in different clinical modalities come in the form of questions, albeit many are more complex than what our dataset can ever address. Previous work has used the patient history sentences and the 14 CheXpert image-level labels (X) from reports \cite{} to derive a VQA-like CXR dataset automatically. The dataset was used to train a VQA model that attempts to interactively answer just one type of questions, 'is there {X} in the image?' given the clinical history and prior answers from the model for the same image \cite{}. With our graph dataset, some of the clinically interesting questions that we could ask and automatically derive include, given {prior model answers}: 1) Does the CXR have {X}?, 2) Where is {X}?, 3) Is an anatomy {A} {normal, abnormal}?, 4) Does {A} have {X}?, 5) Is the finding {X} at {A} related to disease {Y} given {patient history}?, 6) Is {X} {improved, worsened (or new), no change} at {A} since the previous CXR?, etc. Besides giving a window for clinical experts to assess the consistency of of answers from a trained model (thereby earning some trust), the clinical application potential for a well trained interactive read system such as this is to be imagined even by the clinical community.

\textbf{Extraction of CXR knowledge graph from reports using NLP}:
The NLP pipeline consists of a sequence of several modules that harness prior curated CXR lexicons (a dictionary of N phrases for XX concepts) and a CXR ontology to derive the documented radiology knowledge from each CXR report. The curation methodology for this resource, which uses a human-in-the-loop concept expansion NLP engine \cite{}, has been previously described in detail \cite{}. The subset of CXR ontology used for constructing this scene graph dataset contains XX concepts (each mapped to the corresponding UMLS CUI), N unique phrases for concept detection (dual validated by 2 radiologists), YY parent-child relations, Z attribute to ``possible'' anatomical objects relations, and ZZ attribute to ``must have'' anatomical objects relations. The CXR scene graph construction NLP modules are described below:

1) The report pre-processing module sorts sentences in each report document into one of three sections -- preliminary report, history, and final report -- and to uniquely index each sentence for all the reports. This sectioning requirement is particular for the MIMIC reports we worked with. Regex was used to identify all potential section trigger phrases from the MIMIC CXR reports. Trigger phrases referring to the three target sections were kept and grouped for sorting sentences by keyword inclusion downstream. Each CXR report document is tokenized into a list of sentences using primarily NLTK, but we also added custom regex patterns to improve sentence tokenization performance on the MIMIC CXR reports (e.g. regex to remove de-identification tags). SpaCy was used to pre-chunk sentences into segments based on conjunction words and customed noun phrase grouping. The offsets for the sentence segments were saved for later anatomy location detection purposes. For each report, the output from this module consists of a list of sequentially ordered sentences, each mapped to an unique sentence index, its section and sentence segment offsets.

2) Concept and context detection module. A previously described rule-based concept extraction algorithm is used to extract CXR concepts from each sentence in the preliminary or final report sections \cite{}. %(Algorithm \ref{alg:concept-extraction}). %not enough time for pseudocode
Table \ref{tab:define_nodes_edges} documents the range of nodes (with their radiology semantic categories) and edges in the CXR report knowledge graphs extracted by this module that are included in the final scene graph dataset. % some of this can probably go in supplementary material

3) The anatomical location detection module identifies the laterality (left and/or right) and the relevant anatomical location (e.g. right upper lung zone) for each described attribute. However, often for brevity, radiologists do not always specifically document all the location information of an attribute if that information is part of general medical knowledge. This is almost always true when attributes are negated in the report (e.g. ``No pneumothorax."). However, affirmed attributes can also have missing documented location information (e.g. ``There is background COPD."). For these instances, we relied on the CXR ontology, constructed in collaboration with a radiologist, to fill in the default medically known anatomical location(s) for the described attribute (e.g. COPD -> left lung and right lung). 
%Algorithm \ref{alg:location-detection} describes this location detection module. %not enough time for pseudocode
% Our algorithm currently only deals with anatomy detect at individual sentence levels. However, there are occasions where the anatomical location information for an attribute may be described only in the previous sentence(s) or sometimes even in the previous report. 

4) The Scene graph consistency module is previously described in section \ref{}. There are two rounds of consistency checking and corrections in our pipeline -- one round after the sentence level concept extraction module, and another round after the attributes have been related to their respective anatomical locations. These logical checks corrects most inconsistencies that we are aware of in the scene graphs. At the sentence level, the algorithm is simply ``if a child attribute is true (affirmed/present), then the parent attribute must also true" even if not specifically described. At the anatomical location level, we additionally implemented several more custom logical checks: 
    \begin{itemize}
        \item[*] If an attribute is related to a anatomical location not in its ``possible" list in the CXR ontology, then the relation between the location and the attribute is removed.
        \item[*] If an attribute is not related to a ``must have" anatomical location in the CXR ontology, then the relation is added.
        \item[*] If a location is related to any affirmed anatomical finding or disease attribute(s), then the attribute ``abnormal" should also be related to the location.
        \item[*] If a location is related to any children attribute of ``lung opacity", then the attribute ``lung opacity" should be related to the location. 
        \item[*] Abnormal and normal attributes that co-occur with tubes and lines attributes at the same anatomical locations are filtered out on purpose. We opted to just describe tubes and lines attributes' relations with the anatomical locations that they can be observed in for each study -- and not conclude anything about their placement issues. Technically, the NLP pipeline is currently not evaluated for detecting the relative placement position of the tubes or lines to an anatomical location (e.g. how many centermeters above or below the carina for endotracheal tubes). Clinically, for most types of tubes or lines, correct placement depends on both the anatomical location of its tip as well as the clinical indication for its placement, which may not be a piece of information available to radiologists at the time of report creation. 
    \end{itemize}

5) Comparison relation extraction module: We targeted three main types of visual change relations documented by radiologists in reports: 1) improved (or resolved), 2) worsened (or new), and 3) no change. A dictionary of phrases for each of the comparison relations are curated using the same human-in-the-loop concept expansion engine used to construct the CXR lexicons \cite{}. These comparison cues are detected at the sentence level along with all other CXR concepts. Currently, the comparison relations for the different anatomical locations are only extracted for the final scene graph JSONs if 1) the current CXR exam order is second or later, and 2) if the anatomical location also contains other attribute(s) that are in the anatomical finding, disease or technical assessment categories. Overall, the comparison relations are intended to be interpreted as {anatomical location A at study T} has/had {improved, worsened, no change} compared to {anatomical location A at study T-1} with respect to an  attribute. 

6) The scene graph assembly module assembles the output from the NLP modules described above with the output (bounding box coordinates) from a separate CXR anatomy object detection pipeline to construct a final scene graph JSON for each image. For each CXR report, all described attributes are grouped to the level of anatomical locations so that in the final JSON, each anatomical locations may be described by multiple ordered report sentences. Additionally, the sentence sections and cues for the chronicity and severity (to be interpreted as measures of certainty) of the attributes are kept in separate JSON fields. However, where possible, these JSONs are constructed to closely follow Visual Genome's dataset structure. We provide more detailed descriptions of these CXR scene graph JSONS in the Data Records section.

\hideseg{
\begin{algorithm}[H]
\SetAlgoLined
\KwResult{Write here the result }
 initialization\;
 \While{While condition}{
  instructions\;
  \eIf{condition}{
   instructions1\;
   instructions2\;
   }{
   instructions3\;
  }
 }
 \caption{CXR concept and context detection algorithm}
 \label{alg:concept-extraction}
\end{algorithm}
}

\hideseg{
\begin{algorithm}[H]
\SetAlgoLined
\KwResult{Write here the result }
 initialization\;
 \While{While condition}{
  instructions\;
  \eIf{condition}{
   instructions1\;
   instructions2\;
   }{
   instructions3\;
  }
 }
 \caption{Anatomical location detection algorithm}
 \label{alg:location-detection}
\end{algorithm}
}

% this is what we wrote for MICCAI
%The Chest ImaGenome dataset builds on the works of \cite{wu2020automatic,wu2020ai} to fill this gap by using a combination of rule-based text-analysis and atlas-based bounding box extraction techniques to structure the anatomies and the related pathologies from 217,417 report texts and frontal images (AP or PA view) from the MIMIC-CXR dataset \cite{johnson2019mimic}. In summary, the text pipeline \cite{wu2020ai} first sections the report and retains only the finding and impression sentences. Then it uses a prior curated CXR concept dictionary (lexicons) to identify and detect the context (negated or not) for name entities required for labeling the 18 anatomical regions and 9 CXR pathology labels from each retained sentence. The pathology labels are associated with the anatomical region described in the same sentence with a natural language parser, SpaCy \cite{spacy}, and clinical heuristics provided by a radiologist was used to correct for obvious pathology-to-anatomy assignment errors (e.g. lung opacity wrongly assigned to mediastinum). Finally the pathology label(s) for each of the 18 anatomical regions from repeated sentences are grouped to the exam level. A separate anatomy atlas-based bounding box pipeline extracts the coordinates from each frontal images for the 18 anatomical regions \cite{wu2020automatic}.

\textbf{Extraction of bounding box coordinates for anatomy objects in each CXR image (scene)}:
Extracting the bounding box coordinates of the anatomical locations (objects) in the Chest ImaGenome dataset was performed in stages. The range of anatomical location descriptions in CXR reports was determined by a concept and vocabulary expansion exercise performed across a corpus of 200,000 MIMIC-III CXR reports using a bottom concept expansion engine \cite{}. Based on this analysis, we extended the anatomical zones that an Bbox extraction pipeline from prior work can extract from 6 zones \cite{} to 36 anatomical zones, 29 of which are selected for inclusion in the final Chest ImaGenome dataset \ref{tab:define_nodes_edges}. 

The Bbox extraction pipeline first extracts 14 free-form anatomies using an UNet CXR segmentation model, which was trained on 150 mostly normal frontal CXR images sampled from multiple CXR datasets \cite{} and annotated by a radiologist. A small set of template Bbox annotations was manually created by a radiologist for 13 of the frontal CXRs to derive the average affine ratios between the different anatomical zones. These ratios and several textbook radiology heuristics (e.g. how to estimate the position of the carina from other larger nearby anatomical structures) are used to derive the 36 bounding boxes from the 14 anatomical segmentation masks. This Bbox pipeline was then run on all of the frontal (AP and PA view) MIMIC CXR images to automatically extract the anatomical bounding boxes for the bulk of the Chest ImaGenome dataset.

To reduce the number of failed bounding boxes from the first Bbox extraction pipeline, we sampled 1048 images (with and without diseases) from the dataset to have their bounding boxes be manually validated and, if necessary, corrected. This small Bbox-level ground truth dataset was then use to train a FasterRCNN object detection model that is only used to correct the lungs and mediastinum related bounding boxes from the prior Bbox extraction pipeline if they are missing or if their sizes are less than 50\% of what is expected (judging by the average area for different bounding boxes from the overall dataset). Finally, after both Bbox extraction steps, 180 CXRs out of the whole dataset still had missing bboxes for key CXR anatomies (e.g. lungs and mediastinum). These CXRs were manually reviewed and annotated. XX were added back to the dataset and YY were excluded for being a non-CXR image, lateral view images, or unreadable. Figure \ref{fig:flow_chart} illustrates what was eventually included in the Chest ImaGenoe dataset as compared to the source MIMIC-CXR dataset.
